# Supplementary material for: QuantumEyes: Towards Better Interpretability of Quantum Circuits
Source: arXiv:2311.07980 source file (2023-11-14)
Supplement: Supplementary file 1 [file appendix.tex]

\onecolumn

\section{Interviews in the Preliminary Study}
\label{sec:appen4question}

To carefully inform the designs, we conducted an in-depth preliminary study to collect feedback for the design requirements.
Specifically, we divided the study into two sessions, \textit{i.e.}, the interview and the prototype test. 
We listed all the questions we asked in the interview process, as shown in Tab.\ref{table:3}.
The feedback from the questions is used to implement the visualization system prototype.
All participants were presented with the same questions and were asked to answer the questions in a think-aloud manner.

\begin{table}[htbp]
\caption{%
The pre-defined questions used in the preliminary study for the session of the design requirement collection. 
}
\centering
% \begin{tabular}{c|p{0.8\columnwidth}}
\begin{tabular}{c|p{0.8\columnwidth}}
\hline
Q1                      & What property of quantum circuits do you mostly use in your routine tasks?                          \\ \cline{2-2} 
Q2                      & Which part of a quantum circuit do you think is most difficult to understand?                       \\ \cline{2-2} 
Q3                      & Which component of quantum circuits do you think is most useful for people to understand a circuit? \\ \cline{2-2} 
Q4                      & How to understand the measured result of a quantum circuit?                                         \\ \cline{2-2} 
Q5                      & What is your expected way yo explain quantum gates?                                                 \\ \cline{2-2} 
Q6                      & Which aspects do you think visualization can help you with for quantum circuit interpretability?    \\ \cline{2-2} 
\multicolumn{1}{l|}{Q7} & How to lower the learning costs for domain users to use a tailored tool?                            \\ \hline
\end{tabular}
\label{table:3}
\end{table}

\section{Bloch Sphere}

A Bloch Sphere, as shown in Fig. \ref{fig:appen1}, is a widely-used representation to visual quantum states in the quantum computing community.
Bloch Sphere utilizes a point on a unit sphere to represent a quantum state, where the angles with the axes indicate the \textit{amplitudes} of the quantum state. Despite the prevalence, Bloch Sphere has several limitations which need to be improved urgently:

\begin{itemize}
    \item Bloch Sphere cannot support the multi-qubit state visualization, while the entanglement of multiple qubits is the power to achieve the quantum advantages.

    \item Bloch Sphere cannot visualize the probability of each basis state intuitively - the only way to acquire the probabilities from Bloch Sphere is a manual calculation based on the angles with the coordinates.

    \item Bloch Sphere is a 3D geometrical visualization, which has been proven to perform worse than two-dimensional counterparts when conducting precise measurements.
\end{itemize}

In this work, we propose a novel geometrical visualization named \designName, which can address the above issues through multiple correlated 2D shapes.
In addition, a \designName\ can mitigate the scalability issue based on the geometry principle using user interactions.

\begin{figure}[htbp]% specify a combination of t, b, p, or h for top, bottom, on its own page, or here
  \centering % avoid the use of \begin{center}...\end{center} and use \centering instead (more compact)
  \includegraphics[width=0.4\columnwidth]{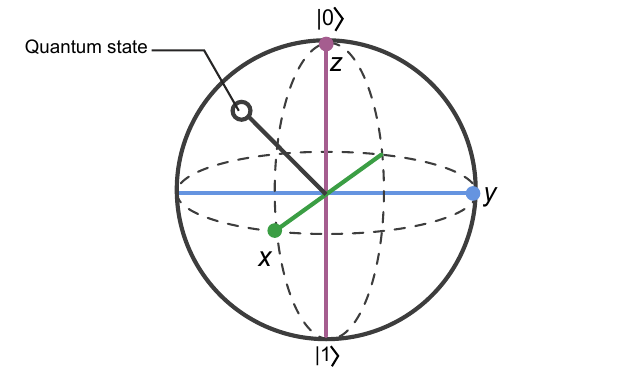}
  \caption{The graphical illustration of Bloch Sphere.}
  \label{fig:appen1}
\end{figure}

\section{Usage of Dandelion Chart Package}

According to the suggestions we collected from the post-study interview, several experts recommend we pack the methods of building a \designName\ and publish it as a public-available web-based package.
To this end, we published the package named \textit{``dandelion\_chart''}\footnote{\designURL{}} to the online software registry, enabling a quick build for developers to visualize a specific quantum state.

The exported function to build \designName\ requires six parameters, \textit{i.e.}, the array of the \emphasize{state vector} of the quantum state, the array of the \emphasize{names} of all basis states, the \emphasize{container} to draw the design, the \emphasize{size} of the chart, the \emphasize{position} of the chart, and a \emphasize{factor} to resize the circles in the chart. We also publish a function named \textit{``generateStates()''} to generate all necessary state names based on the number of digits. For more detailed usage instructions and examples, please refer to the package homepage.

\section{System Interface}
\label{sec:appen4system}

The system interface of \toolName\ is shown in Fig. \ref{fig:appen4}.
Specifically, the system consists of four views, an original quantum circuit, and a control panel.

The summary view of a quantum circuit, as shown in the Probability Summary View, provides an overview of the measured probability. 
For a more detailed analysis of the basis states across each step, the State Evolution View is available. 
The effects of quantum gates and the transformation of qubit states are explained in \revise{Gate Explanation View}. 
By combining State Comparison View with the geometrical visualization of \designName{}, users can gain a better understanding of the measured probability in terms of amplitudes.
Additionally, the original quantum circuits, the quantum computing users are most familiar with, flatten the learning curves of using the visualization system \toolName.

\begin{figure}[htbp]% specify a combination of t, b, p, or h for top, bottom, on its own page, or here
  \centering % avoid the use of \begin{center}...\end{center} and use \centering instead (more compact)
  \includegraphics[width=0.9\columnwidth]{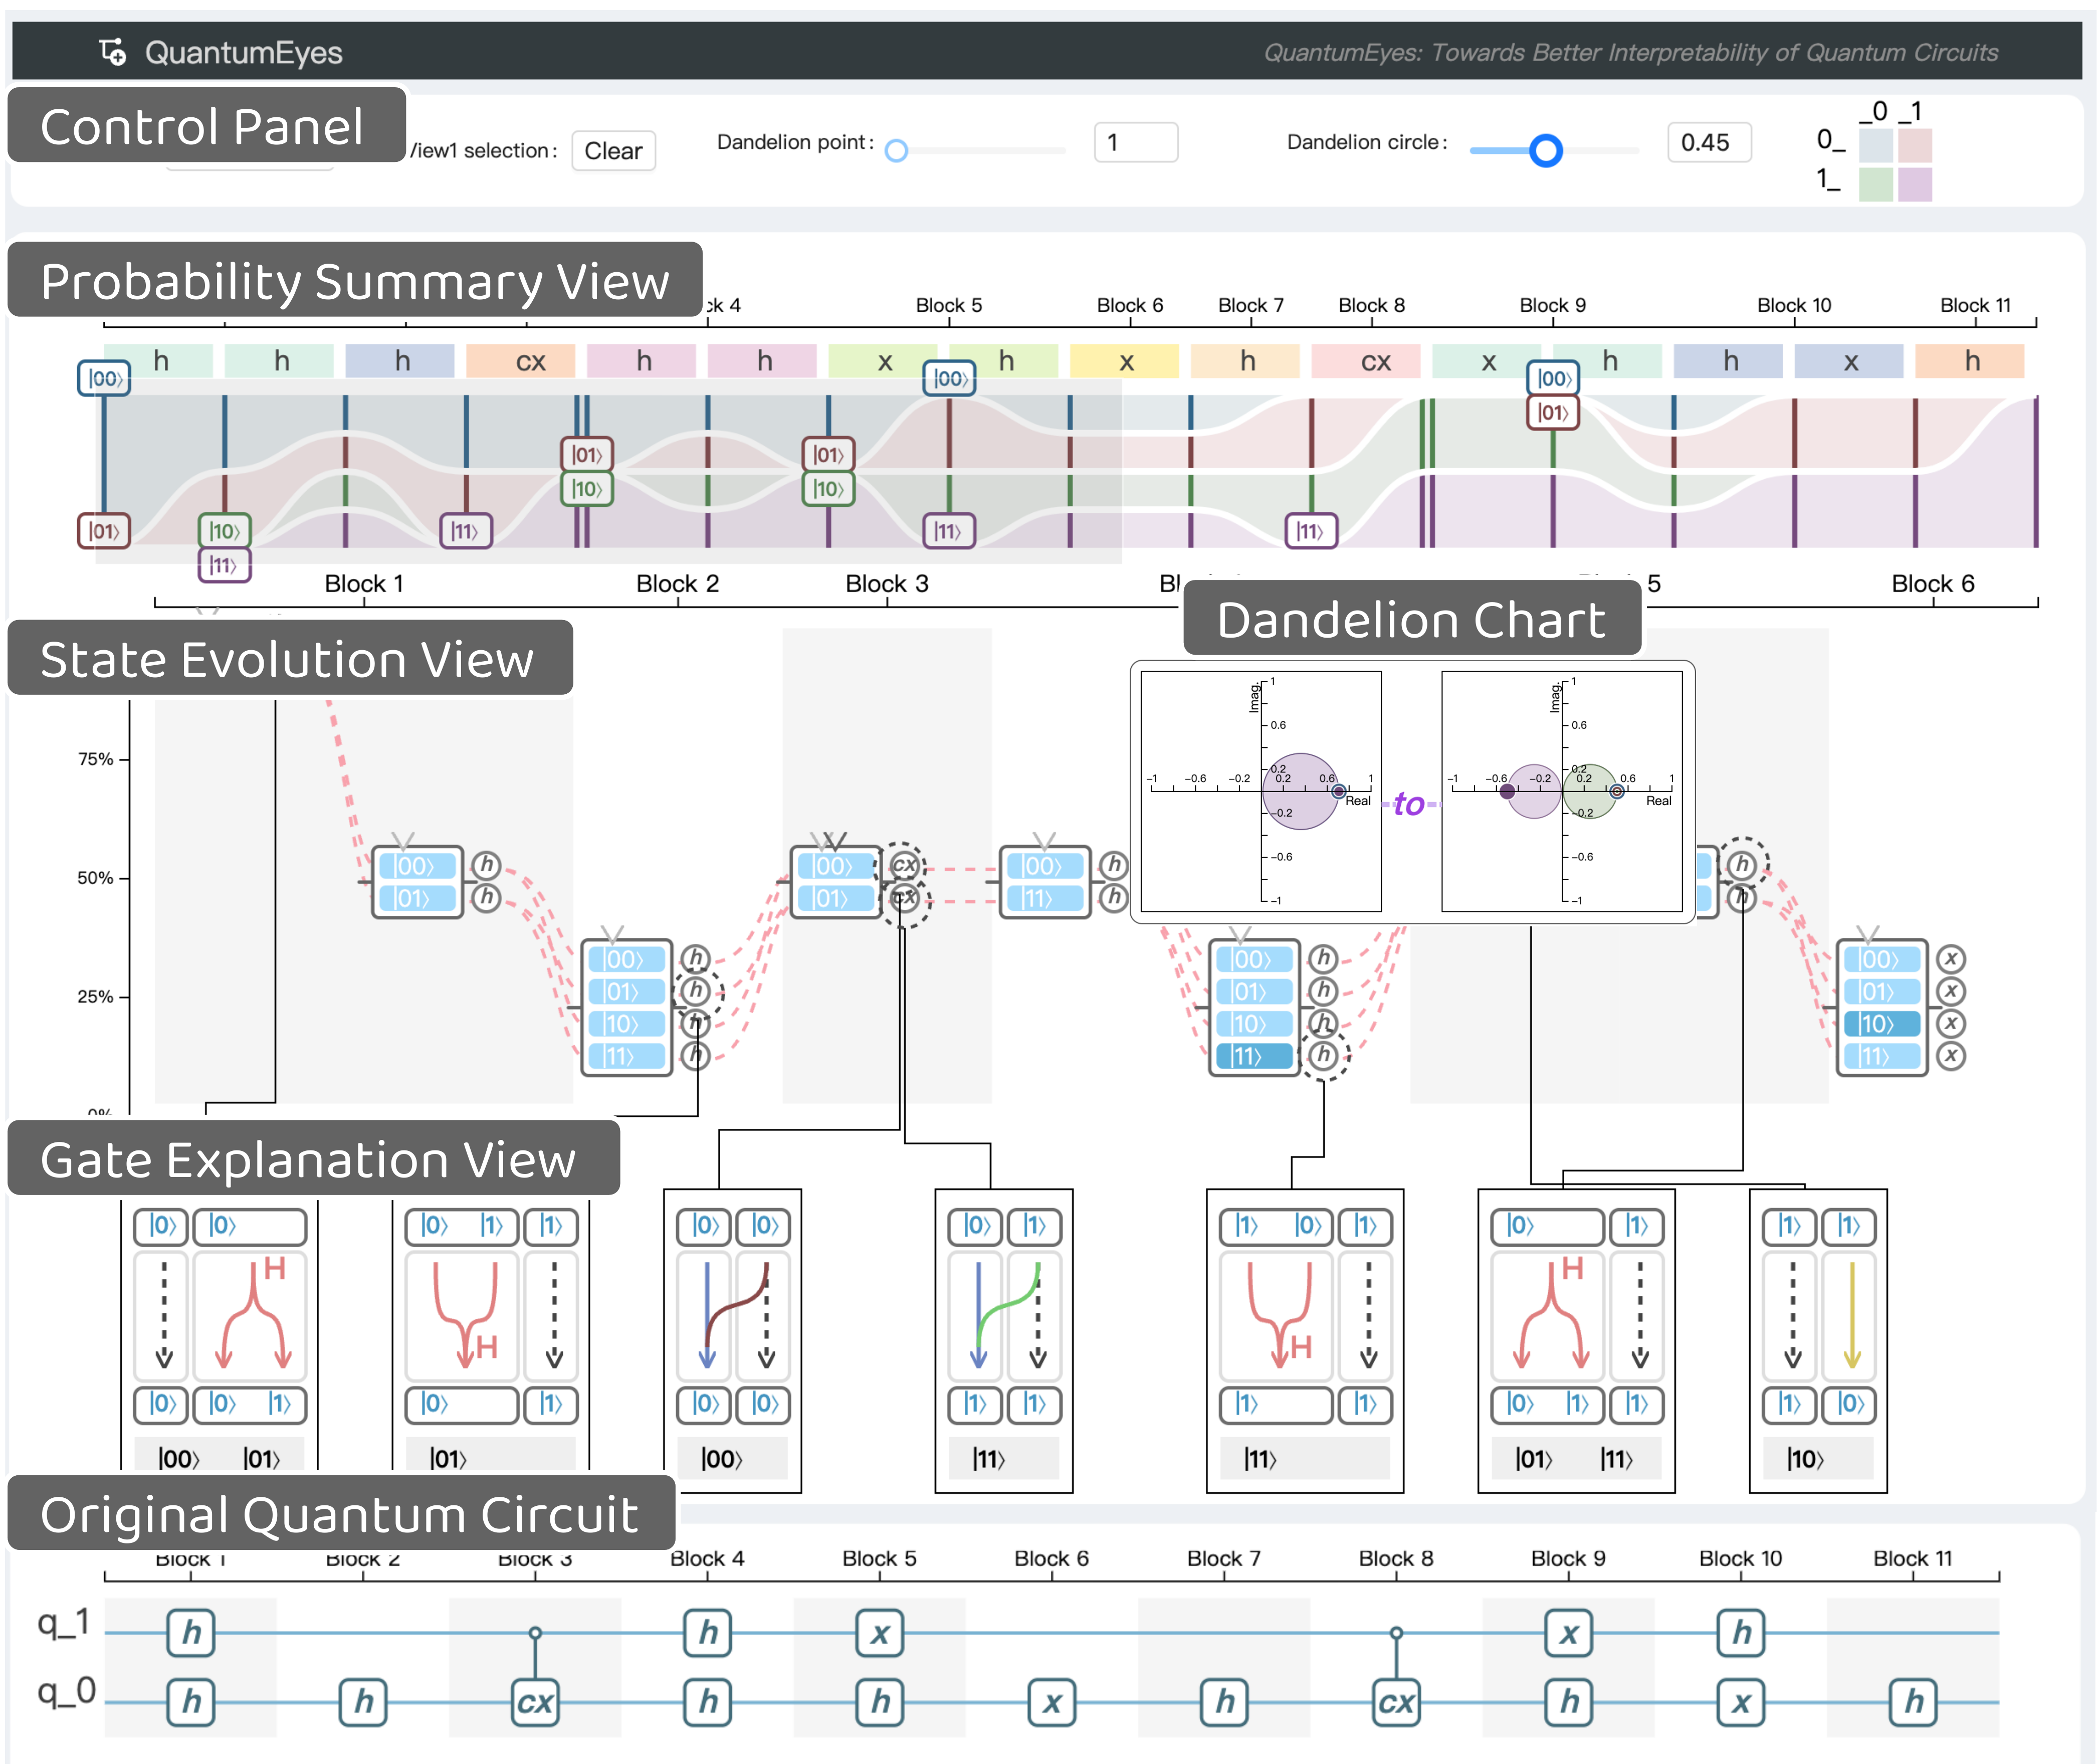}
  \caption{
\revise{The system interface of \toolName, which consists of four views, an original quantum circuit, and a control panel.}
  }
  \label{fig:appen4}
\end{figure}

\section{Matrix Decomposition}
\label{sec:appen4matrixDecom}

As shown in Fig. \ref{fig:appen3}, we illustrate the matrix decomposition using an example of a transformation of the CNOT gate.
First, the state vector of the initial quantum state is $(0, 1, 1, 0)^{\mathrm{T}}$, which can be split into the sum of the two basis states, \textit{i.e.}, $(0, 1,0, 0)^{\mathrm{T}}$ and $(0, 0, 1, 0)^{\mathrm{T}}$. 
Meanwhile, the basis states of the above two state vectors are $\ket{01}$ and $\ket{10}$.
After the transformation of the CNOT gate, the above two basis states are converted into $\ket{11}$ and $\ket{10}$, respectively.
Thus, we completed the matrix decomposition by manipulating the basis states separately using the quantum gates.

\begin{figure}[htbp]% specify a combination of t, b, p, or h for top, bottom, on its own page, or here
  \centering % avoid the use of \begin{center}...\end{center} and use \centering instead (more compact)
  \includegraphics[width=0.7\columnwidth]{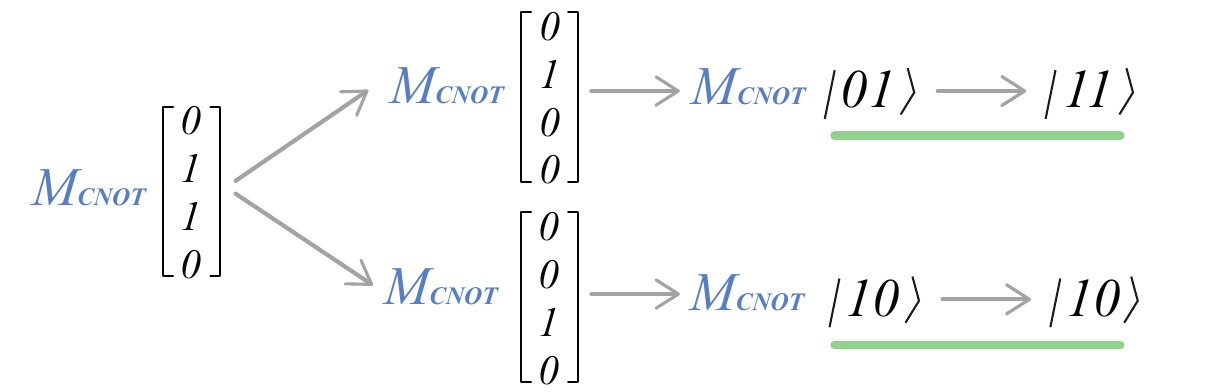}
  \caption{
  The illustration of matrix decomposition.
  We use a transformation of the CNOT gate acting on States $\ket{01}$ and $\ket{10}$ as an example. 
  The matrix represents the state vector of the basis states of a quantum state.
  }
  \label{fig:appen3}
\end{figure}

\section{Introduction of Commonly-used Quantum Gates}
\label{sec:appen4gate}

To illustrate the operations of various quantum gates, we proposed several visual designs to depict the transformation acting on the qubit state.
As shown in Fig. \ref{fig:appen2}, we briefly introduce the commonly-used quantum gates regarding the abbreviation, visualization in \revise{Gate Explanation View}, matrix representation, and the symbol used in the quantum circuit diagram.
Specifically, we implemented the operations of six types of quantum gates, including two types of Hadamard gates, two types of CNOT gates, Not gate, and SWAP gate.

\textbf{Hadamard gate} is a basic quantum gate that operates on a single qubit, transforming it into a superposition state. It is represented by a matrix and when applied to a qubit in the $\ket{0}$ or $\ket{1}$ state, it transforms it into a superposition of the two states. The Hadamard gate is a fundamental building block in quantum algorithms and circuits.

\textbf{CNOT gate}, short for controlled-NOT gate, is a fundamental quantum gate that operates on two qubits, a control qubit, and a target qubit. It performs a NOT operation on the target qubit only when the control qubit is in the $\ket{1}$ state, otherwise, it leaves the target qubit unchanged. The CNOT gate can be represented by a $2 \times 2$ matrix and is often used as a basic building block for various quantum algorithms and circuits.

\textbf{NOT gate}, also known as the Pauli-X gate, is a fundamental quantum gate that operates on a single qubit, flipping its state from $\ket{0}$ to $\ket{1}$ or vice versa. The quantum NOT gate can be represented by a $2 \times 2$ matrix and is a basic building block for various quantum algorithms and circuits. It plays a similar role as the classical NOT gate in classical computing but also has additional properties in the quantum realm, such as being able to create entangled states.

\textbf{SWAP gate} is a fundamental quantum gate that operates on two qubits, allowing them to exchange their states. When applied to two qubits in the states $\ket{a}$ and $\ket{b}$, the SWAP gate transforms them into the states $\ket{b}$⟩ and $\ket{a}$, respectively. The quantum SWAP gate can be represented by a $4 \times 4$ matrix and is a basic building block for various quantum algorithms and circuits. It is often used to implement quantum data exchange and to swap the states of two qubits in quantum registers.

\begin{figure}[t]% specify a combination of t, b, p, or h for top, bottom, on its own page, or here
  \centering % avoid the use of \begin{center}...\end{center} and use \centering instead (more compact)
  \includegraphics[width=\linewidth
  ]{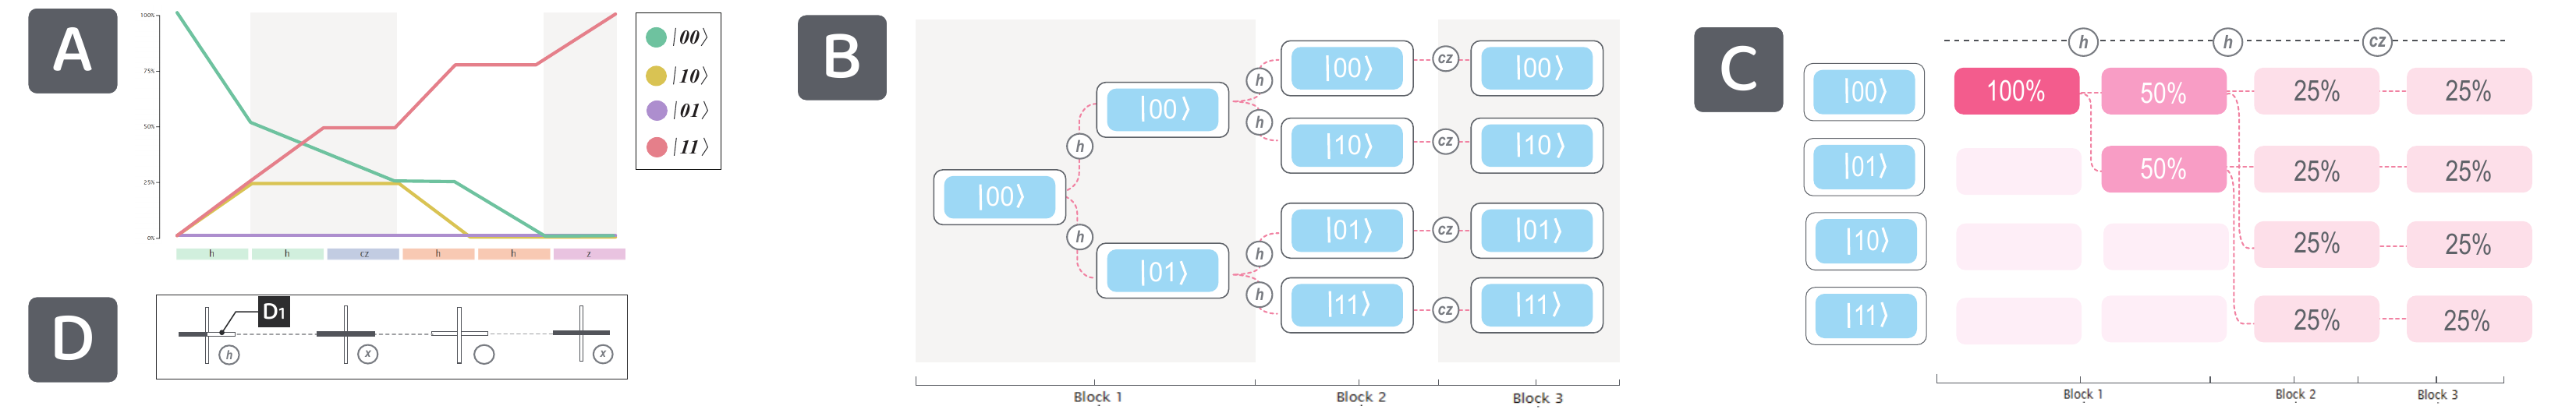}
  \caption{
  The design alternatives of \toolName. 
  (A) The initial visualization summarizes the probability change across each step in the quantum circuit using the multiple-line chart, where the rectangles in the same color on the x-axis indicate the steps in a common block.
  (B) The design 
  allows the analysis of the basis state's evolution via a tree diagram without the awareness of the measured probability of each basis state.
  (C) The visualization approach highlights the probability's change over steps, where the rectangles with different opacity denote the probability of the corresponding basis state.
  (D) The design to depict the qubit state before and after a gate operation, where the rectangles positioned horizontally denote the initial state and the rectangles positioned vertically represent the final state.
  }
  \label{fig:appen4alter}
\end{figure}

\begin{figure}[htbp]% specify a combination of t, b, p, or h for top, bottom, on its own page, or here
  \centering % avoid the use of \begin{center}...\end{center} and use \centering instead (more compact)
  \includegraphics[width=\columnwidth]{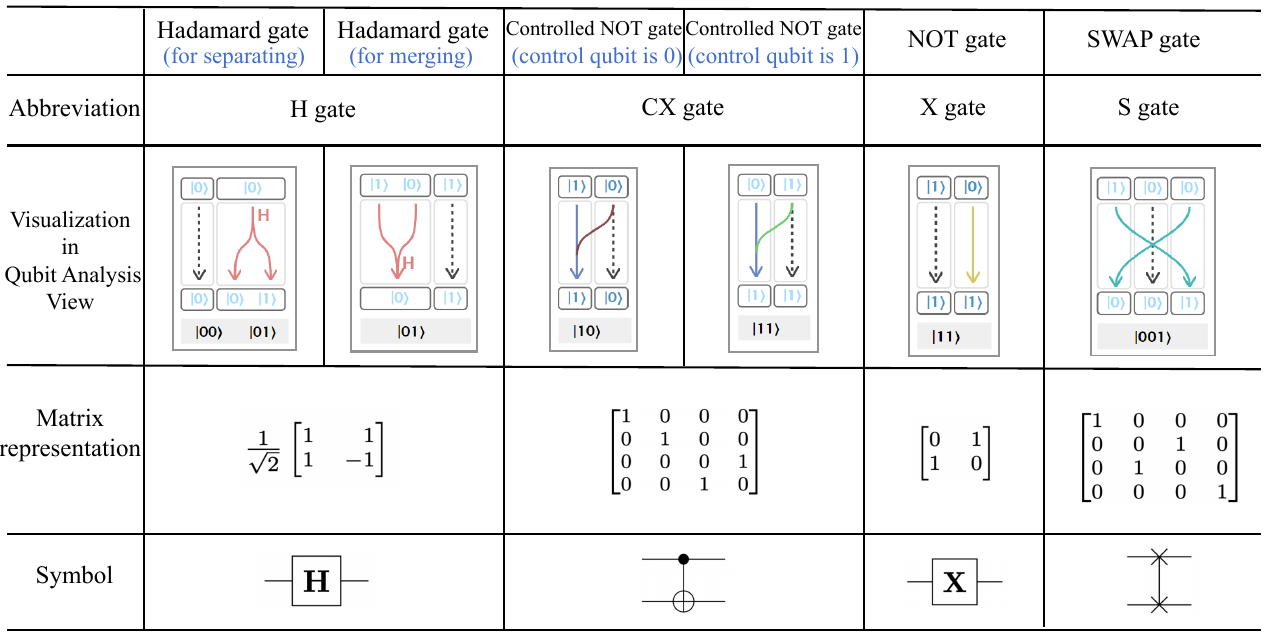}
  \caption{The introduction of six types of commonly-used quantum gates based on their functionality, including two types of Hadamard gates, two types of Controlled NOT gates, NOT gate, and SWAP gate. For a better illustration, we select the two-qubit transformation for the Hadamard gate, Controlled NOT gate, and NOT gate, while we use the three-qubit transformation for the SWAP gate.}
  \label{fig:appen2}
\end{figure}

\begin{table}[!t]
\caption{%
All pre-defined tasks are grouped into two categories, \textit{i.e.}, the effectiveness evaluation of visual designs for global analysis (\textbf{T1-4}) and local analysis (\textbf{T5-6}). \revise{Specifically, T1-4 are designed to evaluate the purpose of each view for global analysis (\textit{i.e.}, T1: overall trend perception, T2-3: gate effect explanation, T4: fine-grained gate explanation regarding individual qubit), and T5-6 are proposed to test dandelion chart's effectiveness of measured probability explanation. }
}
\centering
% \begin{tabular}{c|p{0.8\columnwidth}}
\begin{tabular}{c|p{0.8\columnwidth}}
\hline
T1 & Identify the overall trends of all basis states regarding the measured probability. \\ \cline{2-2} 
T2 & Identify the generation of the basis states via the trace-back analysis.        \\ \cline{2-2} 
T3 & Describe the operations and effects of the quantum gates by comparing the basis states before and after.    \\ \cline{2-2} 
T4 & Explain the effect of the quantum gates from the perspective of the qubit state analysis.            \\ \hline
T5 & Explain how quantum gates change the amplitudes of the basis states.       \\ \cline{2-2} 
T6 & Explain how amplitudes of basis states change the corresponding measured probabilities.             \\ \hline
\end{tabular}
\label{table:1}
\end{table}

\section{Design Alternatives}

\subsection{Probability Summary View}
\label{subsec:view1}
Initially, we attempted to use a multiple-line chart to show the probability change of each basis state in the circuit, as shown in Fig. \ref{fig:appen4alter}\component{A}. However, we encountered problems with the lines crossing over and overlapping, which made it hard to see. The design also didn't make it easy to see the proportion of each basis state's probability. 
In the end, we decided to use a stacked area chart, \revise{which is able to (1) avoid any overlapping between multiple entities, and (2) visually reflect the proportion of each basis state using the fixed height of the vertical coordinate.}

\subsection{State Evolution View}
\label{subsec:view2}
We explored a couple of different design options before landing on the current visual design. 
Initially, we tried using a tree diagram to organize all of the basis states (Fig. \ref{fig:appen4alter}\component{B}), but an expert pointed out that there were no discernible patterns regarding the gate's effect on the states, as they were all located evenly in each step. Next, we tried a design that utilized the opacity of corresponding rectangles to visualize the probability of each basis state (Fig. \ref{fig:appen4alter}\component{C}), while the dotted lines depicted the state evolution. However, we encountered problems with severe line overlapping between adjacent steps, so this design was not scalable. Ultimately, we developed the current design,
\revise{which enables to clustering of the basis state at each step based on their measured probability, making it easy to find the patterns of the quantum circuit and also differentiate the basis states to avoid any visual clutter.}

\subsection{\revise{Gate Explanation View}}
\label{subsec:view3}
We also explored other options where a set of rectangles was used to represent the qubit states (Fig. \ref{fig:appen4alter}\component{D}). A rectangle is colored white if the quantum state is $\ket{0}$, black if it is $\ket{1}$, and half black and half white if it is in a superposition state (Annotation \subcomponent{D\textsubscript{1}}). The initial states were placed vertically, while the final states were placed horizontally. However, this design was not preferred as it only showed the initial and final states without explicitly visualizing the gate operations. 
\revise{Therefore, we use the current visual design with a layout of "before-transformation-after," which can highlight the gate operations process more clearly. The design is more compact to enable the state visualization with more qubits.}

% \subsection{State Comparison View}
% \label{subsec:view4}

\section{Pre-defined Tasks in Expert Interview}
\label{sec:tasks}

We conducted a well-designed expert interview to demonstrate the effectiveness and usability of our visualization system \toolName.
Specifically, we asked each expert to perform the pre-defined tasks and rate the system based on the exploration of the tasks.
All six tasks are categorized into two groups: \textit{i.e.}, the effectiveness evaluation of visual designs for global analysis (\textbf{T1-4}) and local
analysis (\textbf{T5-6}).
We listed all tasks in Table \ref{table:1} for a better illustration.

\vfill

% \section{System Architecture}

% \revise{\ref{fig:2} illustrates the architecture of \toolName, which consists of three tightly-connected modules: 
% (1) data storage module, (2) data processing module, and (3) visualization module.}

% \definecolor{module_storage}{RGB}{159, 168, 69}
% \definecolor{module_processing}{RGB}{159, 183, 172}
% \definecolor{module_visualization}{RGB}{178, 78, 50}

% \begin{figure}[htbp]% specify a combination of t, b, p, or h for top, bottom, on its own page, or here
%   \centering % avoid the use of \begin{center}...\end{center} and use \centering instead (more compact)
%   \includegraphics[width=0.5\columnwidth]{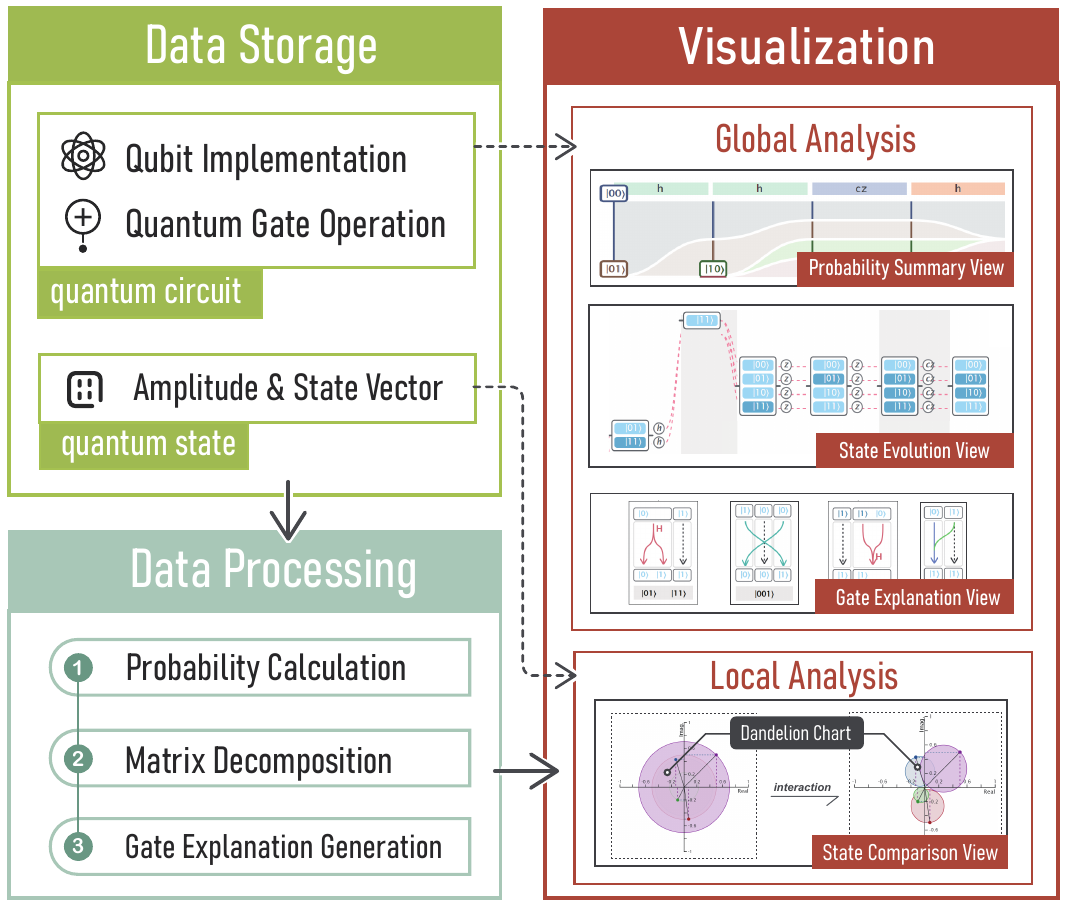}
%   \caption{The system architecture of \toolName\ consists of three modules, i.e, a \textcolor{module_storage}{\textbf{data storage}} module, a \textcolor{module_processing}{\textbf{data processing}} module, and a \textcolor{module_visualization}{\textbf{visualization}} module.}
%   \label{fig:2}
% \end{figure}
